# Supplementary material for: A unified Green's function approach for spectral and thermodynamic properties from algorithmic inversion of dynamical potentials
Source: arXiv:2109.07972 source file (2021-09-16)
Supplement: Supplementary file 1 [file sec_supplemental_material.tex]

%========================
\section{Convergence studies at several densities of the HEG}
\label{sec:Convergence studies at all densities of the HEG}
%========================
In this section we show the convergence studies at all densities of~\cite{thisPaper}. Following the method presented in Secs.~\ref{sec:method_HEG}, and particularly~\ref{sec:numerical_details}, of~\cite{thisPaper} at $r_s=4$, we study stability and convergence of the correlation (total minus Fock) energy per particle at $r_s$ from $1$ to $10$. In Figs.~\ref{fig:SI_totEnecG0W0rs1},~\ref{fig:SI_totEnecG0W0rs2},~\ref{fig:SI_totEnecG0W0rs3},~\ref{fig:SI_totEnecG0W0rs4},~\ref{fig:SI_totEnecG0W0rs5},~\ref{fig:SI_totEnecG0W0rs6},~\ref{fig:SI_totEnecG0W0rs7},~\ref{fig:SI_totEnecG0W0rs8},~\ref{fig:SI_totEnecG0W0rs9},~\ref{fig:SI_totEnecG0W0rs10} we plot the convergence study at the different densities.

\begin{figure}
    \centering
    \includegraphics[width=\columnwidth]{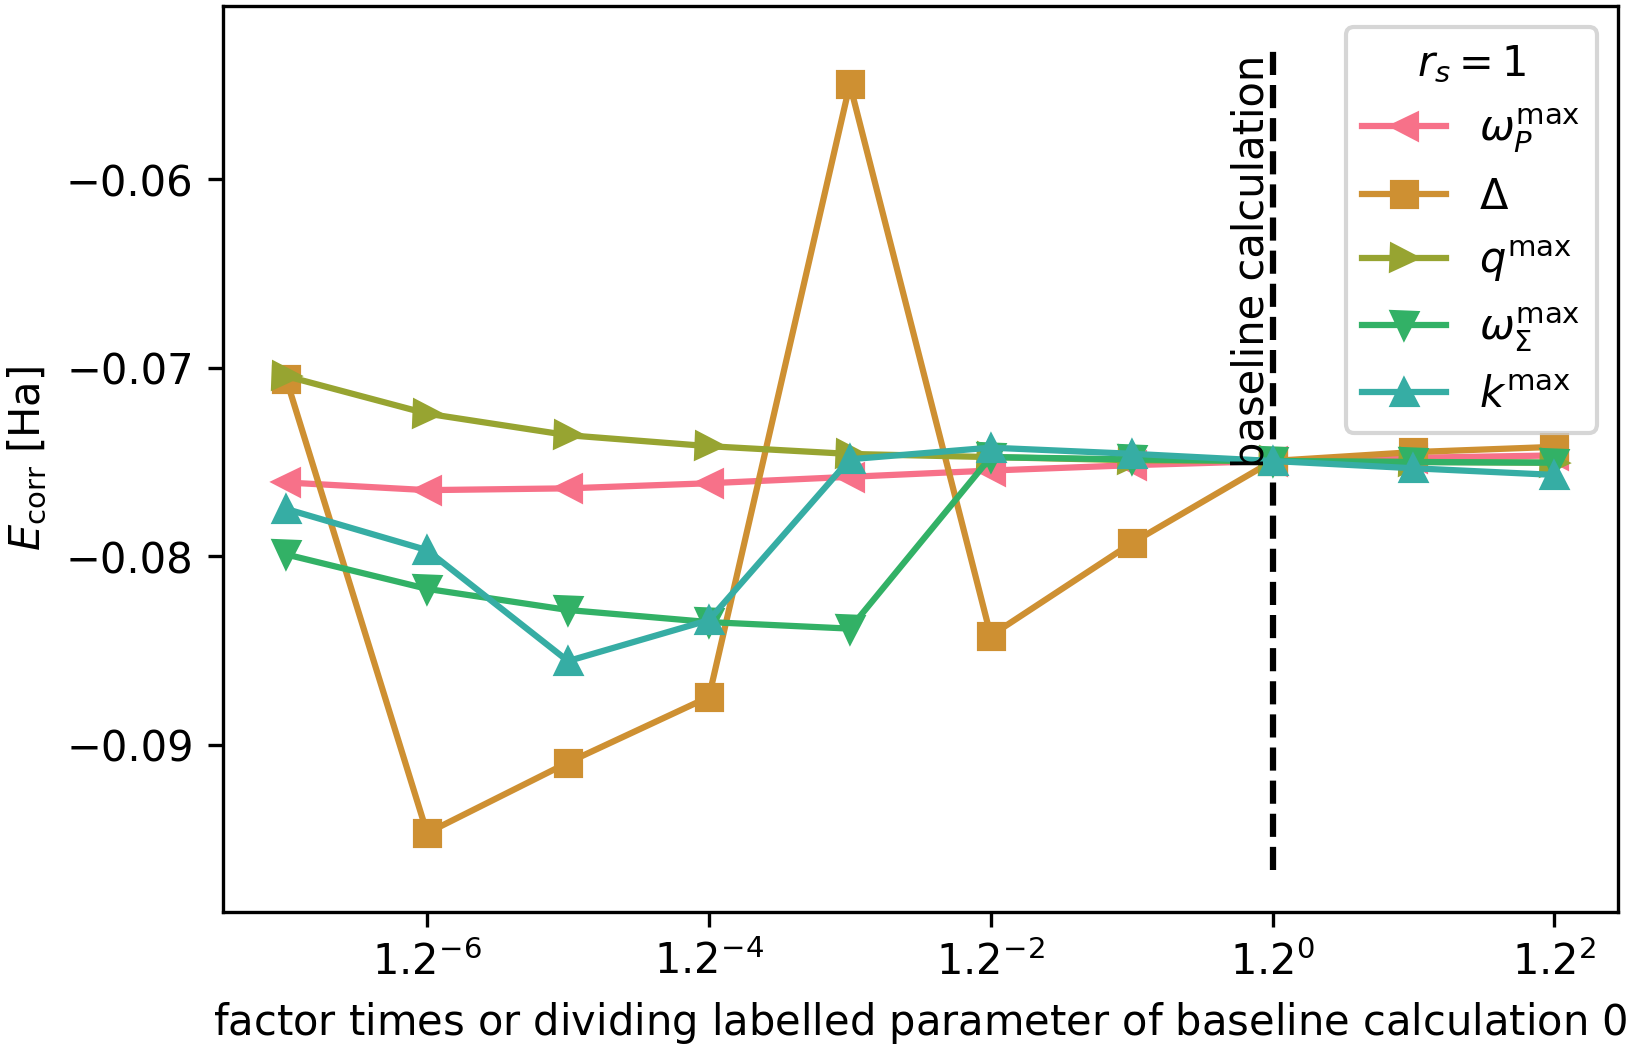}
    \caption{Correlation energy $E_\mathrm{corr}$ convergence study obtained with the Galitzki-Migdal formula using a Green function from a $G_0W_0$ calculation for the HEG at $r_s=1$. See Fig.~\ref{fig:totEnecG0W0rs4} of~\cite{thisPaper} for further reference.}
    \label{fig:SI_totEnecG0W0rs1}
\end{figure}
\begin{figure}
    \centering
    \includegraphics[width=\columnwidth]{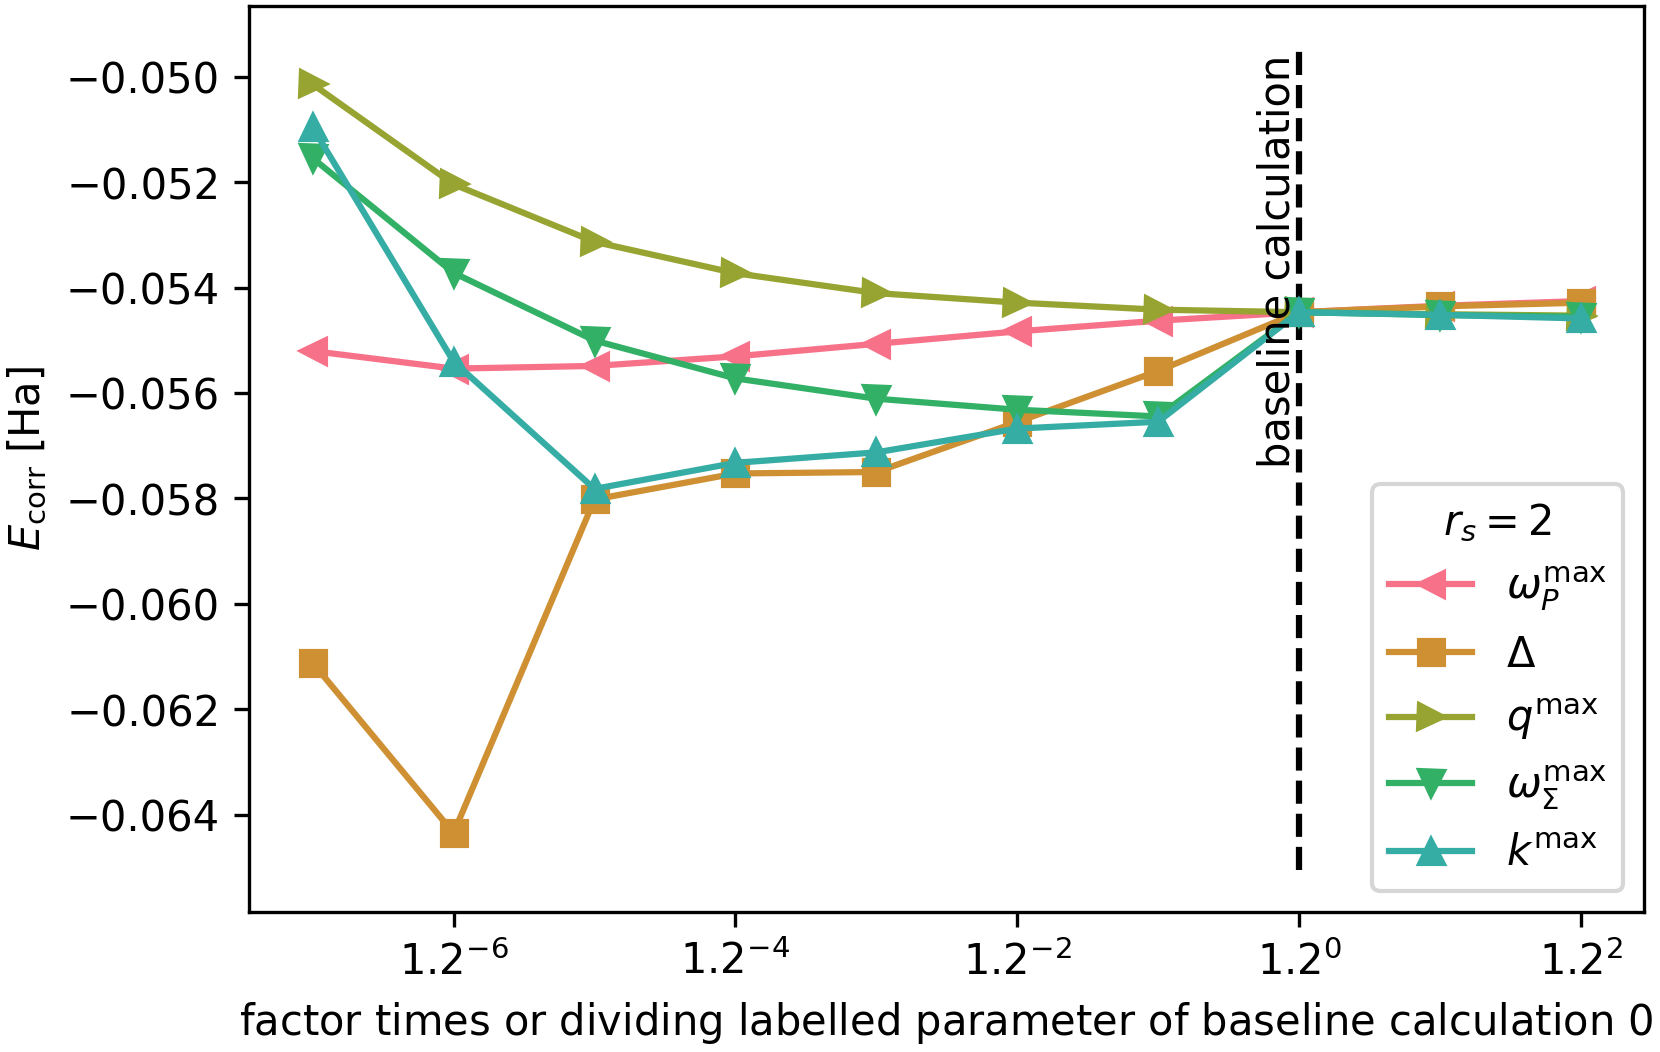}
    \caption{Correlation energy $E_\mathrm{corr}$ convergence study obtained with the Galitzki-Migdal formula using a Green function from a $G_0W_0$ calculation for the HEG at $r_s=2$. See Fig.~\ref{fig:SI_totEnecG0W0rs4} of~\cite{thisPaper} for further reference.}
    \label{fig:SI_totEnecG0W0rs2}
\end{figure}
\begin{figure}
    \centering
    \includegraphics[width=\columnwidth]{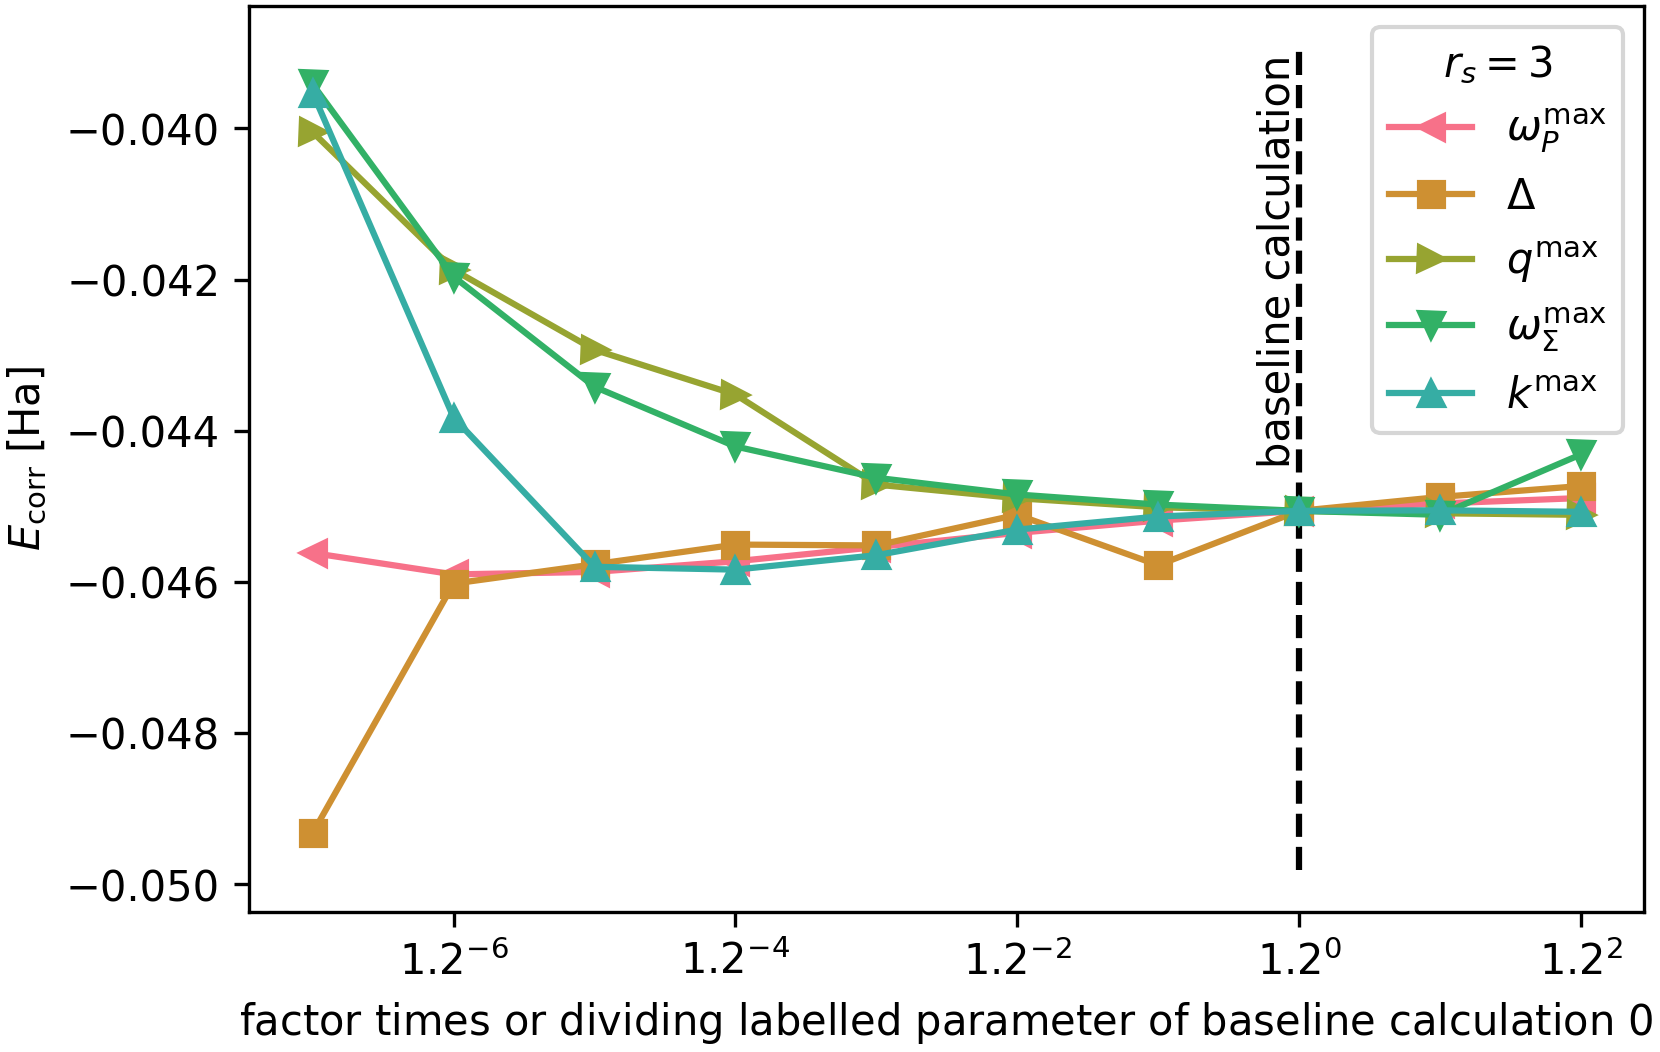}
    \caption{Correlation energy $E_\mathrm{corr}$ convergence study obtained with the Galitzki-Migdal formula using a Green function from a $G_0W_0$ calculation for the HEG at $r_s=3$. See Fig.~\ref{fig:totEnecG0W0rs4} of~\cite{thisPaper} for further reference.}
    \label{fig:SI_totEnecG0W0rs3}
\end{figure}
\begin{figure}
    \centering
    \includegraphics[width=\columnwidth]{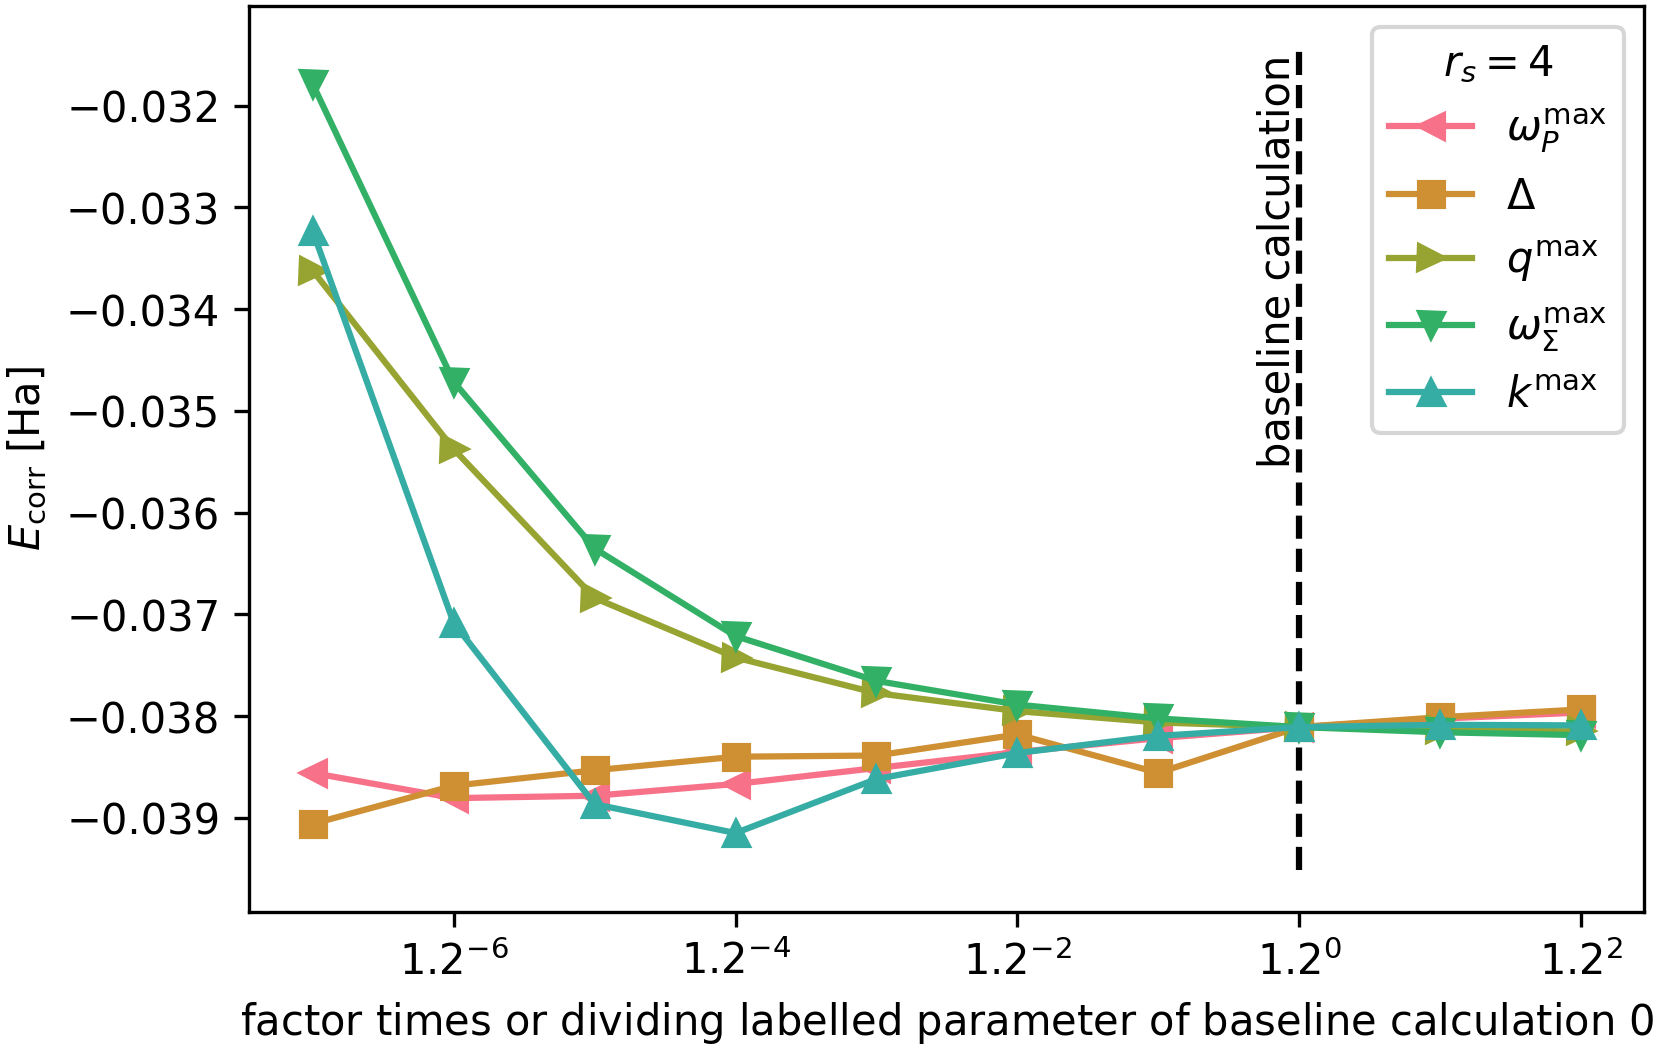}
    \caption{Correlation energy $E_\mathrm{corr}$ convergence study obtained with the Galitzki-Migdal formula using a Green function from a $G_0W_0$ calculation for the HEG at $r_s=4$. See Fig.~\ref{fig:totEnecG0W0rs4} of~\cite{thisPaper} for further reference.}
    \label{fig:SI_totEnecG0W0rs4}
\end{figure}
\begin{figure}
    \centering
    \includegraphics[width=\columnwidth]{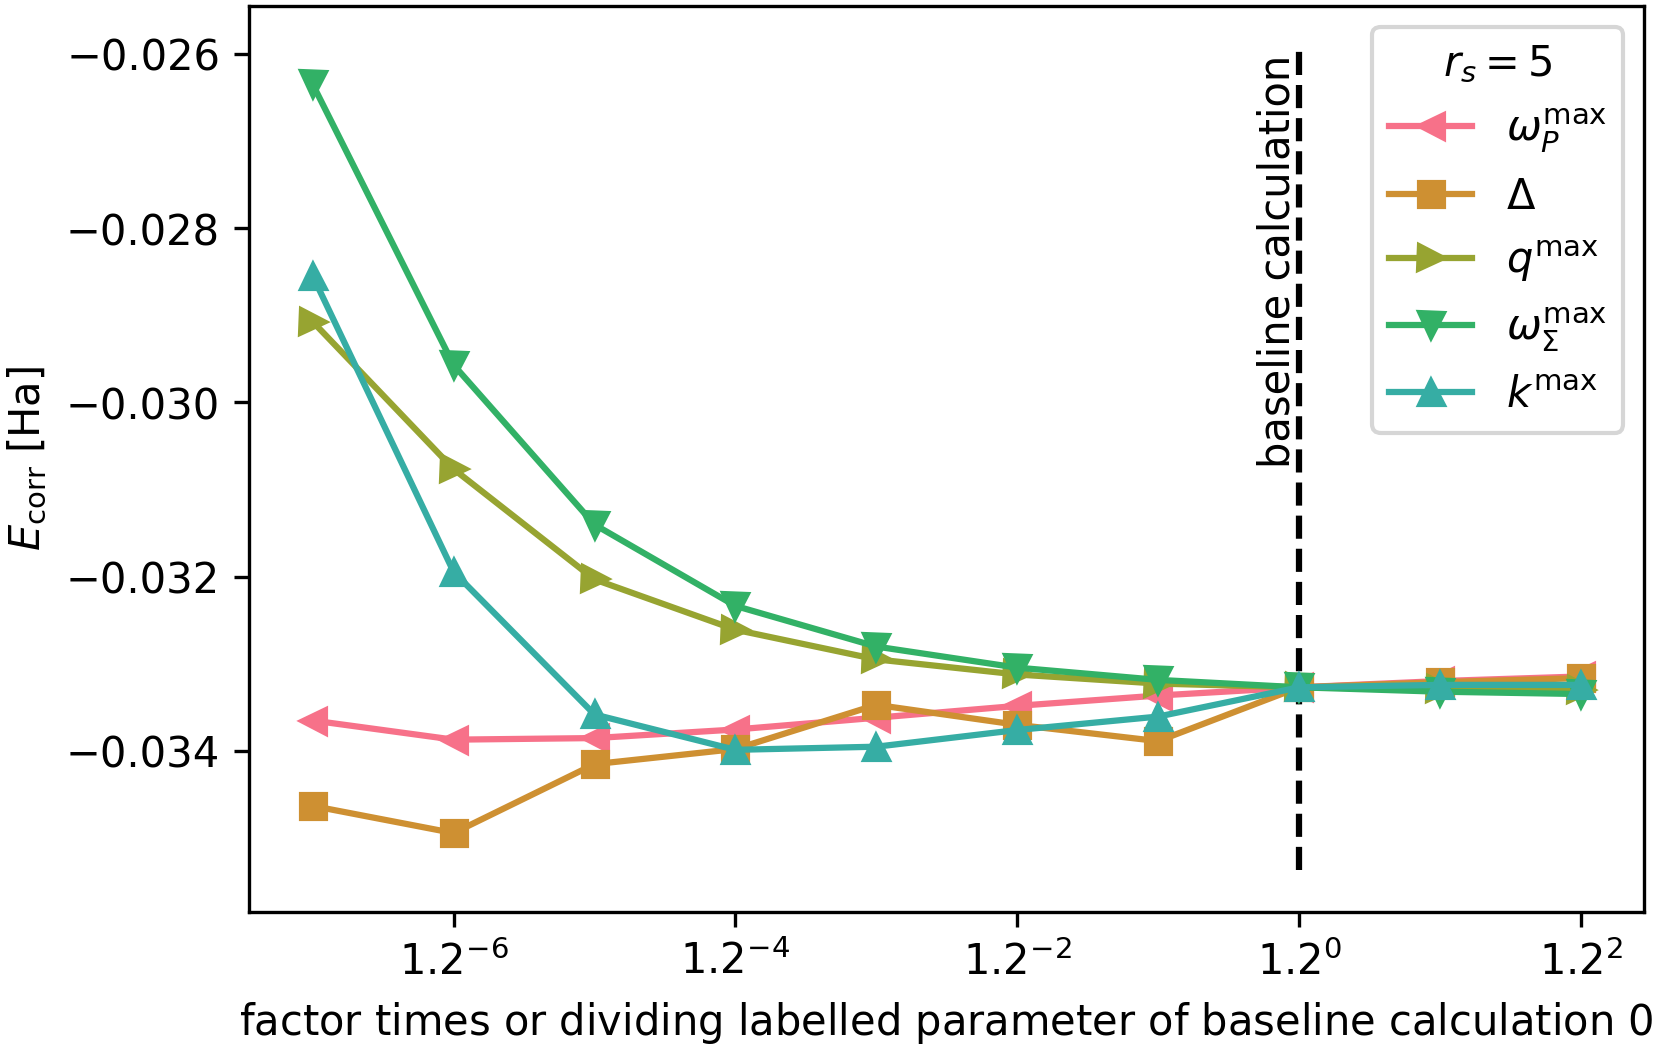}
    \caption{Correlation energy $E_\mathrm{corr}$ convergence study obtained with the Galitzki-Migdal formula using a Green function from a $G_0W_0$ calculation for the HEG at $r_s=5$. See Fig.~\ref{fig:totEnecG0W0rs4} of~\cite{thisPaper} for further reference.}
    \label{fig:SI_totEnecG0W0rs5}
\end{figure}
\begin{figure}
    \centering
    \includegraphics[width=\columnwidth]{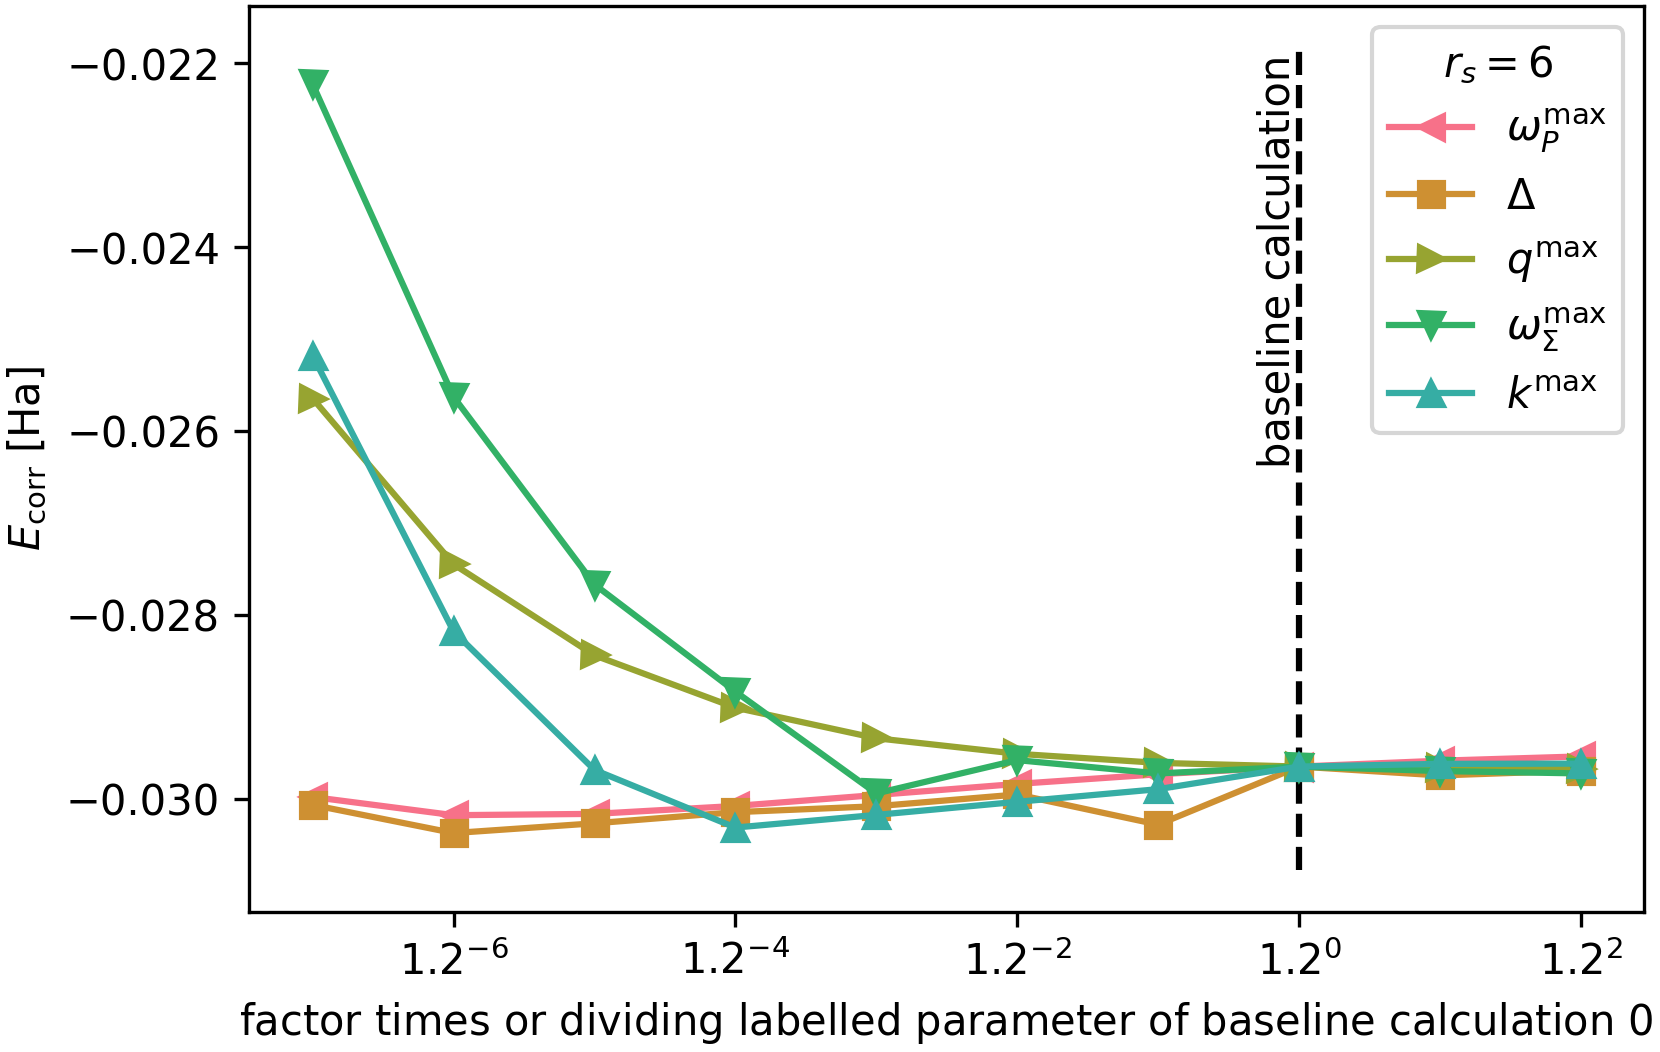}
    \caption{Correlation energy $E_\mathrm{corr}$ convergence study obtained with the Galitzki-Migdal formula using a Green function from a $G_0W_0$ calculation for the HEG at $r_s=6$. See Fig.~\ref{fig:totEnecG0W0rs4} of~\cite{thisPaper} for further reference.}
    \label{fig:SI_totEnecG0W0rs6}
\end{figure}
\begin{figure}
    \centering
    \includegraphics[width=\columnwidth]{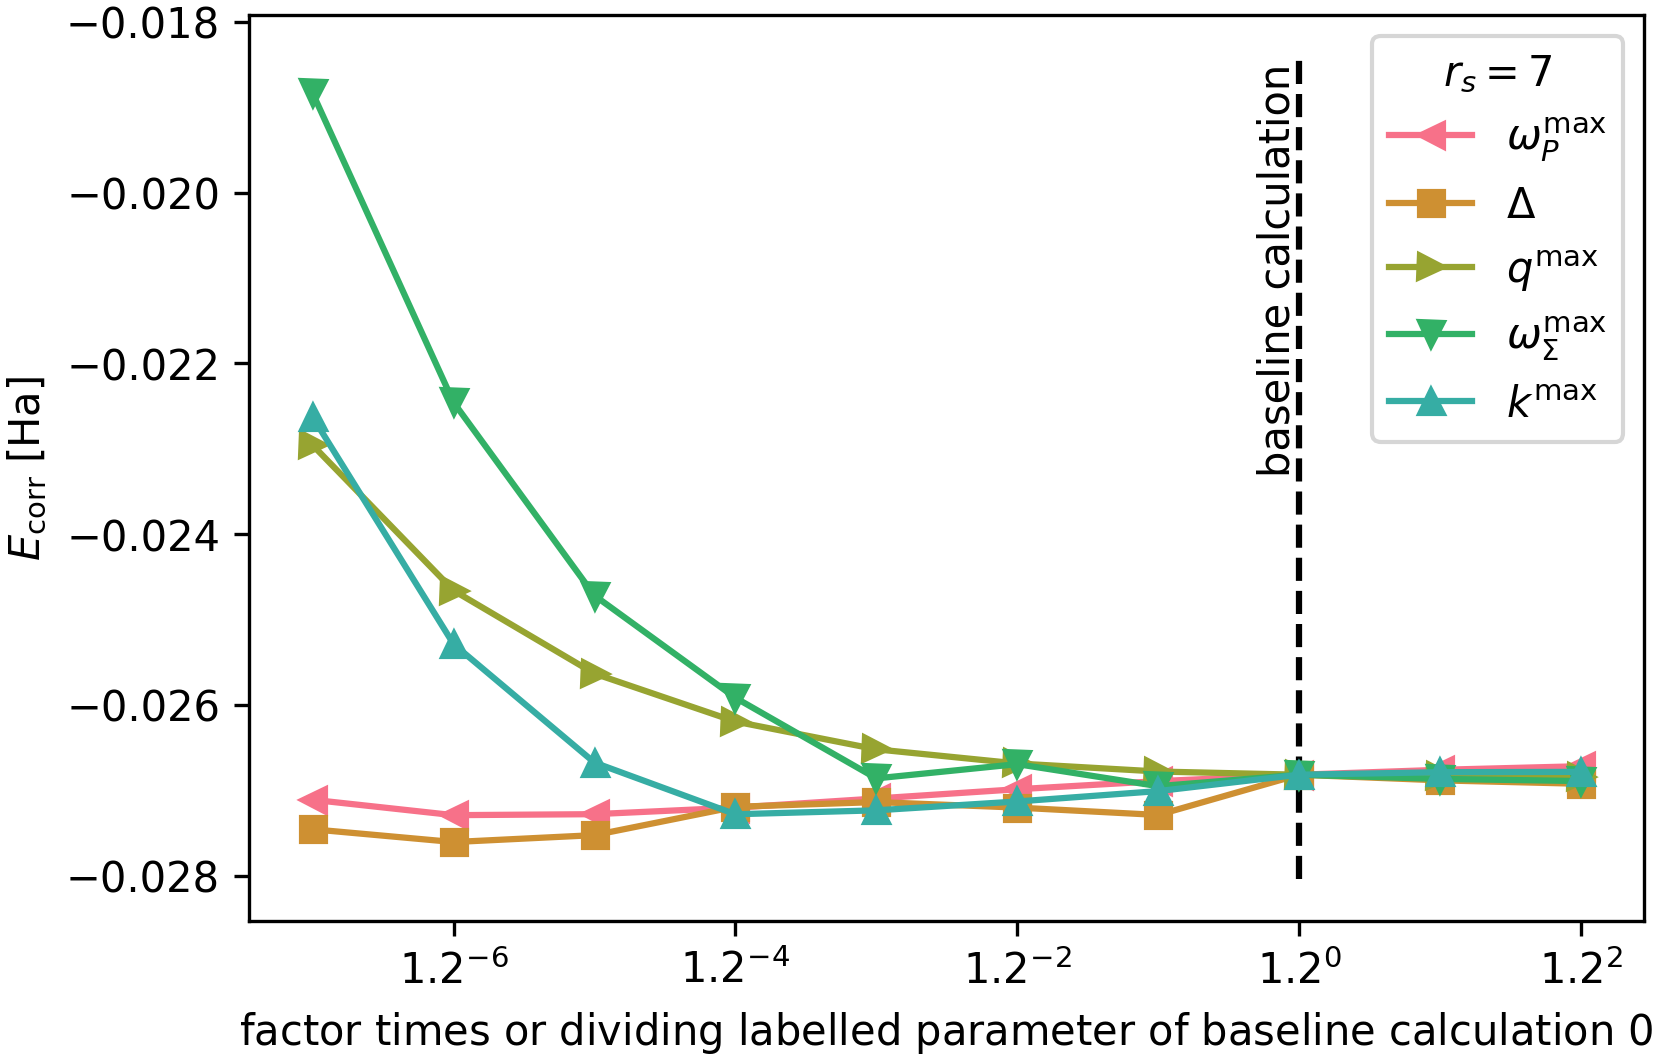}
    \caption{Correlation energy $E_\mathrm{corr}$ convergence study obtained with the Galitzki-Migdal formula using a Green function from a $G_0W_0$ calculation for the HEG at $r_s=7$. See Fig.~\ref{fig:totEnecG0W0rs4} of~\cite{thisPaper} for further reference.}
    \label{fig:SI_totEnecG0W0rs7}
\end{figure}
\begin{figure}
    \centering
    \includegraphics[width=\columnwidth]{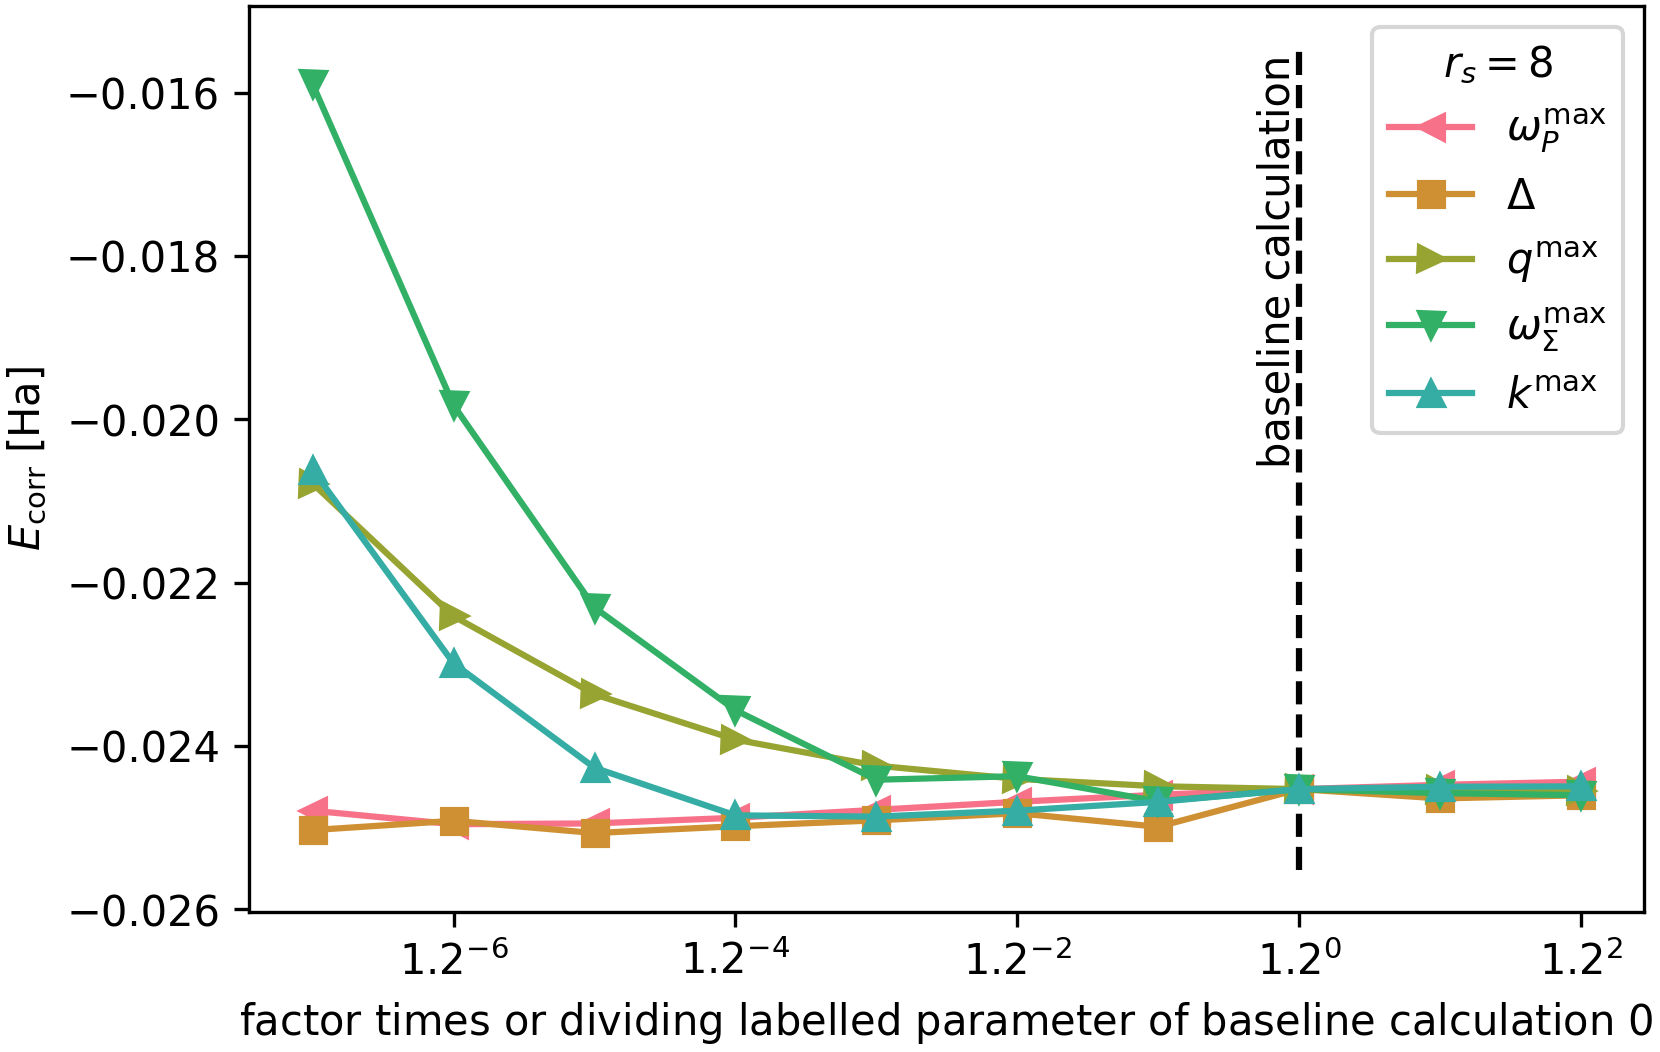}
    \caption{Correlation energy $E_\mathrm{corr}$ convergence study obtained with the Galitzki-Migdal formula using a Green function from a $G_0W_0$ calculation for the HEG at $r_s=8$. See Fig.~\ref{fig:totEnecG0W0rs4} of~\cite{thisPaper} for further reference.}
    \label{fig:SI_totEnecG0W0rs8}
\end{figure}
\begin{figure}
    \centering
    \includegraphics[width=\columnwidth]{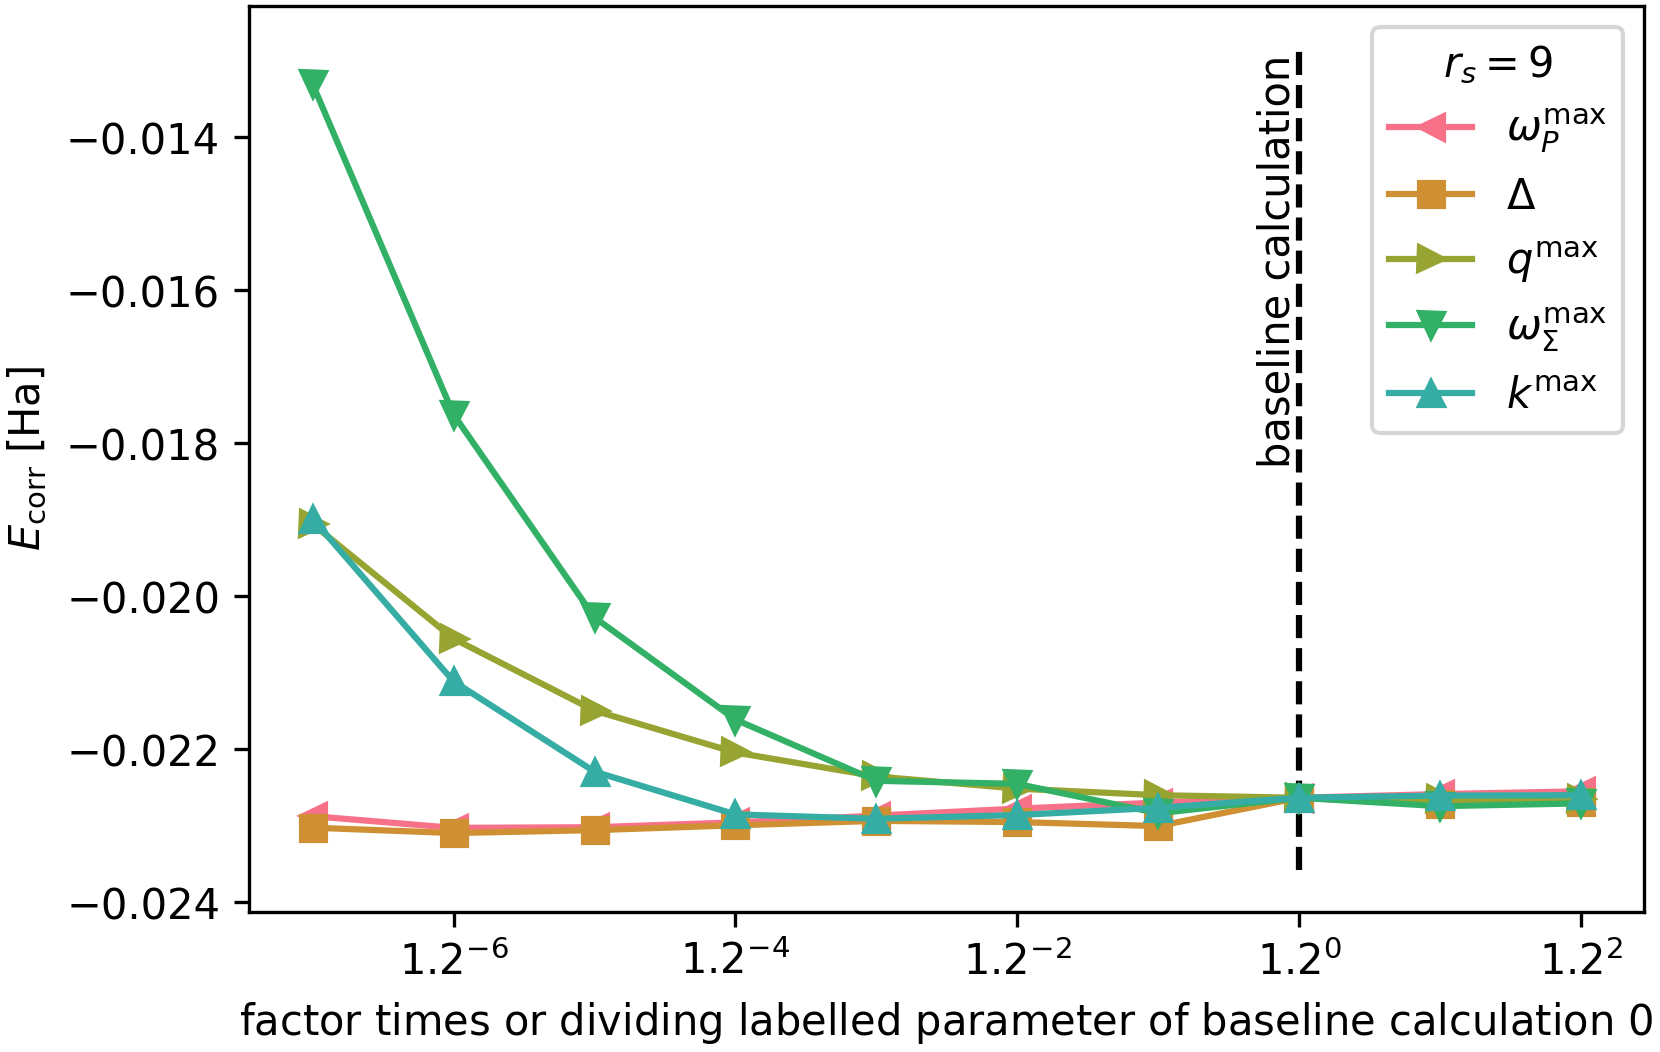}
    \caption{Correlation energy $E_\mathrm{corr}$ convergence study obtained with the Galitzki-Migdal formula using a Green function from a $G_0W_0$ calculation for the HEG at $r_s=9$. See Fig.~\ref{fig:totEnecG0W0rs4} of~\cite{thisPaper} for further reference.}
    \label{fig:SI_totEnecG0W0rs9}
\end{figure}
\begin{figure}
    \centering
    \includegraphics[width=\columnwidth]{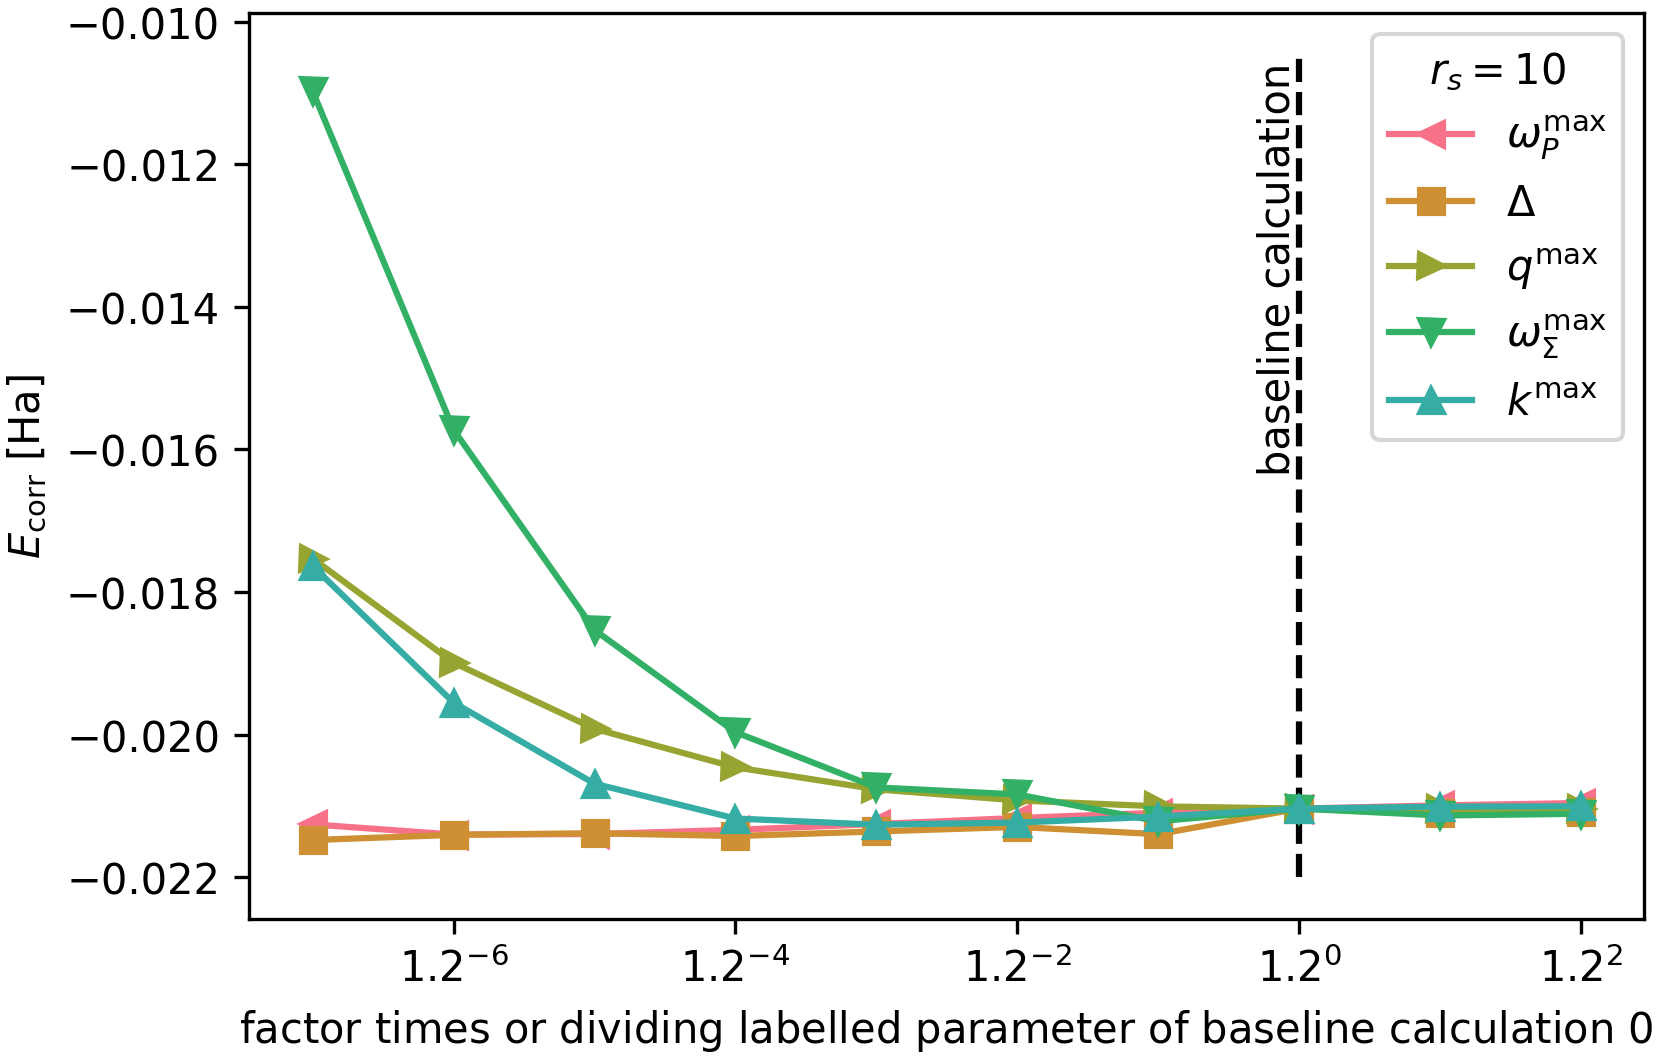}
    \caption{Correlation energy $E_\mathrm{corr}$ convergence study obtained with the Galitzki-Migdal formula using a Green function from a $G_0W_0$ calculation for the HEG at $r_s=10$. See Fig.~\ref{fig:totEnecG0W0rs4} of~\cite{thisPaper} for further reference.}
    \label{fig:SI_totEnecG0W0rs10}
\end{figure}
